# Supplementary material for: Coding4Games: Can Modern Coding Agents Play Modern Video Games?
Source: arXiv:2611.31974 source file (2026-11-24)
Supplement: Supplementary file 1 [file appendix.tex]

% Unified appendix: edit this file; all required media are in assets/.
\providecommand{\appendixassetroot}{Sec/appendix/assets}
\section{Implementation Details}
\label{app:implementation}
This appendix describes the implemented game-tool interface, recorded initialization procedure, and server-side scoring pipeline.

\subsection{Game and Submission APIs}
\label{app:apis}
The coding agent accesses server-controlled game tools through an MCP adapter. Both the coding agent and the generated program observe gameplay through screenshots only. Generated programs can invoke the corresponding tools through a supplied client connected to the authenticated local bridge. These are benchmark interaction and lifecycle APIs, rather than game-engine APIs exposing semantic actions such as selecting a card or buying an item. General-purpose shell and filesystem operations are supplied by the coding CLI separately.

Table~\ref{tab:api-details} lists the registered tools. Development exposes all nine tools; independent testing exposes only \texttt{game.observe}, \texttt{game.step}, \texttt{game.stop}, and \texttt{bench.status}. In independent testing, the server starts the episode and launches the selected artifact, so the program cannot create additional episodes or change the submitted artifact through these tools.

\begin{table}[htbp]
\centering\small
\caption{\textbf{Registered benchmark APIs.} D: Development stage; T: Test stage. Optional arguments are described in the text; signatures summarize the principal inputs.}
\label{tab:api-details}
\setlength{\tabcolsep}{4pt}\renewcommand{\arraystretch}{1.16}
\begin{tabular}{@{}>{\raggedright\arraybackslash}p{.27\linewidth}>{\raggedright\arraybackslash}p{.08\linewidth}>{\raggedright\arraybackslash}p{.61\linewidth}@{}}
\toprule
Tool & Phase & Inputs and effect \\
\midrule
\texttt{game.start} & D & \texttt{mode} (set to \texttt{stepped} in the current protocol), optional \texttt{max\_tics}: initialize a fresh episode and return its identifier and initial observation. \\
\texttt{game.observe} & D, T & Optional \texttt{episode\_id}: capture an observation, or return the settled result of an ended episode. \\
\texttt{game.step} & D, T & Structured \texttt{actions}, or \texttt{controls} and \texttt{tics}: execute physical inputs in a stepped episode and return an observation and timing receipt. \\
\texttt{game.stop} & D, T & Optional \texttt{episode\_id}: stop the episode, settle its score, and return the result. \\
\texttt{bench.status} & D, T & No arguments: report budget consumption and session status. The final-test response excludes the development episode history. \\
\texttt{bench.replay} & D & \texttt{uid}, \texttt{start}, \texttt{end}, optional \texttt{every}: retrieve frames from a completed episode recording without advancing the game. \\
\texttt{submission.save} & D & \texttt{path}, \texttt{entrypoint}, optional description and dependencies: archive an immutable executable candidate and return its identifier. \\
\texttt{submission.run} & D & \texttt{id}, optional \texttt{max\_tics}: self-test a saved candidate in a fresh episode, using the development sandbox and shared budget. \\
\texttt{submission.finish} & D & \texttt{id}: select a saved artifact and end development. Early submission is accepted; exhausting the development budget is not required. \\
\bottomrule
\end{tabular}
\end{table}

\paragraph{Physical actions and timing.}
In keyboard/mouse mode, \texttt{game.step} accepts an ordered list of \texttt{click}, \texttt{double\_click}, \texttt{move}, \texttt{drag}, \texttt{scroll}, \texttt{keypress}, and \texttt{wait} actions. Each action specifies a positive duration in game tics. Coordinates refer to a $1280\times768$ observation surface; scrolling uses wheel steps, and dragging specifies a two-point path. In gamepad mode, a call instead specifies physical control tokens and a duration. The two formats cannot be mixed. These controls do not encode game-specific strategies.

The server validates the action batch before execution. Each stepped action resumes the game, delivers the input, releases controls, and pauses the game before returning observations. Receipts distinguish requested and actual tics, executed actions, and truncation due to termination or budget limits. Tics are computed from measured running time at the scenario's configured rate, rather than read from an internal engine clock.

\paragraph{Returned evidence and artifact identity.}
Tool results associate observations and outcomes with episode identifiers, resource use, and available evidence references. During gameplay, \texttt{score} is null rather than zero. After settlement, \texttt{done}, \texttt{complete}, \texttt{outcome\_kind}, and \texttt{end\_reason} distinguish an ended episode from a valid scored result. A successful execution is not itself a submission: saving produces a candidate archive, while finishing explicitly selects its identifier. Independent tests use that selected archive rather than the mutable development directory. If the agent has not yet submitted when it has consumed 70\% of its development budget, it receives a reminder to wrap up development and prepare its final submission. This reminder does not require immediate termination; the agent may continue working within the remaining budget or choose to submit earlier.

\subsection{Recorded Initialization and Fixed Task Starts}
\label{app:initialization}
Every episode follows one server-controlled initialization procedure: prepare the registered task state, cold-start the game, replay a recorded startup sequence, and perform the configured readiness checks before transferring control. This procedure places repeated evaluations at the same designated task entry, such as a fresh run, fixed match, boss encounter, or route. It does not require every game to have the same notion of a ``level,'' nor does it guarantee identical random draws or trajectories.

\paragraph{Recording and replay.}
Menu navigation is prepared in advance as a recorded sequence of physical inputs and waits, stored in the game configuration as \texttt{menu\_skip}. Entries preserve the input parameters, duration, and, where relevant, controller index. The server launches the executable, waits for and focuses the game window, then replays this sequence to enter the registered scenario. Thus, repeated menu navigation is automated by replaying recorded operations; it is not solved anew by the evaluated agent. The recording is an action sequence, not a video used to synthesize gameplay. Scenarios can request open-loop replay; the controller also supports screen-aware replay. Neither introduces a game-playing strategy after control is transferred.

\paragraph{Preparing the initial state.}
Before launch, the server stops the previous game process. When a scenario specifies a reference checkpoint, it restores the corresponding archive into the configured save location, replacing the covered files according to the restore configuration. Otherwise, the preparation hook clears a resumable run where the game has a registered cleanup routine.

\paragraph{Readiness and scope of reproducibility.}
Where configured, the server checks screen text and exact field values before handoff. It inspects the game while paused and advances short pulses when a transition needs to complete, avoiding an unbounded period of gameplay during recognition. Failed configured checks can trigger a cold-start retry and ultimately an initialization error. Window geometry is also configured where required by the scorer. These checks verify selected visible conditions, not a complete internal-state snapshot. Configured checks differ across tasks.

% Evidence gap: do not upgrade configured startup procedures to universal
% validation or identical state/seed claims without scenario acceptance artifacts.

\subsection{External Scoring and Episode Recordings}
\label{app:scoring}
The server constructs a scorer from the scenario's registered implementation and calibration. Scorers operate on captured game images, using OCR for text and numbers or image rules for health bars and result screens. This is distinct from querying a game-engine state oracle, asking the coding agent to self-report progress, or using an agent to judge its own output.

\paragraph{Capture, stop, and settle.}
During gameplay, the environment queues scoring frames in a disk-backed stream using lossless PNG encoding. Episode video recordings provide a separate replay artifact; the scorer does not depend on decoding that compressed video. Once the episode stops, the server settles its score from the retained frames. For trajectory-based scorers, it resets the scorer and processes frames in temporal order:
\begin{equation}
 S_g = \sum_{i=1}^{n}\Delta_g(f_i;z_{i-1}),
\end{equation}
where $f_i$ is a retained frame and $z_{i-1}$ is the scorer's accumulated state, such as previous valid readings or confirmed milestones. The increments are task-specific and can be negative, as in health-difference or route-distance scoring. They are not uniformly rewards for each observed frame.

Snapshot-based scorers instead select a valid retained frame and apply their registered score function to that observation. OCR configurations specify regions, language, and confidence thresholds, while stateful rules reject implausible changes or require confirmation.

\paragraph{Result validity and audit records.}
Settlement occurs after gameplay is halted; its completion does not imply victory. The server records the outcome, consumed resources, termination reason, and available replay and scoring evidence. Scoring, sampling, or cleanup errors can invalidate a result: the public score is then null, with a partial value retained separately where available. Invalid or missing scores are excluded from score aggregation, and the corresponding episodes are not rerun. A missing score is not converted to a valid zero; mean scores are computed over the available valid scores. Online lifecycle checks and final score computation are separate; a visual terminal screen is not universally an automatic episode-stop condition. The retained logs and recordings provide an audit trail for inspecting execution failures and scoring readings.

\section{Game Tasks and Scoring}
\label{app:illustrated-games}
\label{app:game-tasks}
Table~\ref{tab:game-task-details} provides the chapter overview: task objectives, scoring criteria, and interaction demands across the working game suite.

% Task and scoring descriptions updated from author clarification; implementation validation remains separate.
% Working roster: fifteen candidate games; membership and unresolved tasks remain provisional.
\begin{table}[!htbp]
\centering
\scriptsize
\setlength{\tabcolsep}{2.5pt}
\renewcommand{\arraystretch}{1.12}
\newcommand{\gamecell}[2]{\parbox[c]{2em}{\centering #1}\hspace{0.5em}\parbox[c]{\dimexpr\linewidth-2.5em\relax}{\raggedright #2}}
\newcommand{\gameicon}[2]{%
  \gamecell{%
    \includegraphics[width=2em,height=2em,keepaspectratio]
    {\appendixassetroot/#1}%
  }{#2}%
}
\caption{\textbf{Games and evaluation tasks.} The 15 games are grouped by their principal interaction demands, with three games in each category. For each task, we summarize its objective, episode-scoring criterion, and required capabilities.}
\label{tab:game-task-details}
\begin{tabular}{@{}>{\raggedright\arraybackslash}m{0.22\linewidth}>{\raggedright\arraybackslash}m{0.22\linewidth}>{\raggedright\arraybackslash}m{0.22\linewidth}>{\raggedright\arraybackslash}m{\dimexpr0.34\linewidth-6\tabcolsep\relax}@{}}
\toprule
\rowcolor{tableheaderblue}
\textbf{Game} & \textbf{Evaluation Task} & \textbf{Episode Scoring} & \textbf{Capabilities Evaluated} \\
\midrule
\rowcolor{tablegroupgray}
\multicolumn{4}{l}{\textcolor{tabletextgray}{\textbf{\textit{Combat \& Action Timing}}}} \\
\gameicon{steam_2358720.jpg}{Black Myth: Wukong (BMW)} & Fight the Black Bear Guai boss and deplete its health & More boss health depleted earns a higher score & Close combat; dodge timing and boss adaptation \\
\arrayrulecolor{black!18}\specialrule{0.15pt}{3pt}{3pt}\arrayrulecolor{black}
\gameicon{steam_814380.jpg}{Sekiro: Shadows Die Twice (SEK)} & Defeat Gyoubu Oniwa in a two-phase boss fight & Progress through both health phases earns points; full victory earns the maximum & Deflection and posture control; phase adaptation \\
\arrayrulecolor{black!18}\specialrule{0.15pt}{3pt}{3pt}\arrayrulecolor{black}
\gameicon{steam_222420.jpg}{The King of Fighters '98 (KOF98)} & Fight a computer-controlled opponent and deplete its health & More opponent health depleted earns a higher score & Real-time fighting; spacing, defense, and attacks \\
\addlinespace[4pt]
\rowcolor{tablegroupgray}
\multicolumn{4}{l}{\textcolor{tabletextgray}{\textbf{\textit{Strategy \& Resource Planning}}}} \\
\gameicon{steam_2379780.jpg}{Balatro (BAL)} & Build scoring card hands to advance through rounds & Stronger hands and later rounds earn more points & Hand construction; discard, economy, and deck planning \\
\arrayrulecolor{black!18}\specialrule{0.15pt}{3pt}{3pt}\arrayrulecolor{black}
\gameicon{steam_646570.jpg}{Slay the Spire (StS)} & Play from the start of a run and climb as many floors as possible & Deeper floors earn higher scores & Turn-based combat; route, deck, and relic planning \\
\arrayrulecolor{black!18}\specialrule{0.15pt}{3pt}{3pt}\arrayrulecolor{black}
\gameicon{steam_2849080.jpg}{Kingdom Rush 5: Alliance (KR5)} & Defend a fixed level against successive enemy waves & Surviving more waves and preserving lives raise the score; victory adds a bonus & Tower placement and upgrades; wave planning \\
\addlinespace[4pt]
\rowcolor{tablegroupgray}
\multicolumn{4}{l}{\textcolor{tabletextgray}{\textbf{\textit{3D Sports \& Precision Control}}}} \\
\gameicon{steam_1551360.jpg}{Forza Horizon 5 (FH5)} & Drive from a fixed start toward a designated destination & Getting closer to the destination earns more points & Road navigation; steering, throttle, and recovery \\
\arrayrulecolor{black!18}\specialrule{0.15pt}{3pt}{3pt}\arrayrulecolor{black}
\gameicon{steam_2290180.jpg}{Riders Republic (RR)} & Perform ski tricks to earn as many points as possible & Successful tricks increase the in-game score & Spatial control; timing and trick execution \\
\arrayrulecolor{black!18}\specialrule{0.15pt}{3pt}{3pt}\arrayrulecolor{black}
% NBA 2K25: recorded points-only evaluation; calibrated outcome detection is absent.
\gameicon{steam_2878980.jpg}{NBA 2K25 (NBA25)} & Score and defend in a 1,000-tic Blacktop one-on-one episode & +15 per own point; -5 per opponent point; no active victory bonus & 3D basketball; movement, shooting, and defense \\
\addlinespace[4pt]
\rowcolor{tablegroupgray}
\multicolumn{4}{l}{\textcolor{tabletextgray}{\textbf{\textit{Movement \& Timing}}}} \\
\gameicon{steam_11020.jpg}{TrackMania Nations Forever (TM)} & Race the A02 course, reaching the finish or going as far as possible & Distance rewards unfinished runs; faster finishes earn more & High-speed control and trajectory optimization \\
\arrayrulecolor{black!18}\specialrule{0.15pt}{3pt}{3pt}\arrayrulecolor{black}
\gameicon{steam_1942280.jpg}{Brotato (BRO)} & Survive successive enemy waves and collect materials & Later waves drive the score; collected materials add points & Movement and combat; upgrade and resource allocation \\
\arrayrulecolor{black!18}\specialrule{0.15pt}{3pt}{3pt}\arrayrulecolor{black}
\gameicon{steam_238460.jpg}{BattleBlock Theater (BBT)} & Collect gems to unlock the exit and complete a platforming level & Gems reward progress; finishing adds speed and yarn bonuses & Platforming; jump timing and route finding \\
\addlinespace[4pt]
\rowcolor{tablegroupgray}
\multicolumn{4}{l}{\textcolor{tabletextgray}{\textbf{\textit{Multi-step Task Execution}}}} \\
\gameicon{steam_728880.jpg}{Overcooked! 2 (OC2)} & Prepare and serve orders by switching between two chefs & The final kitchen score rewards completed orders; episodes that do not complete the task receive no score, even if they end normally & Order planning; chef switching and coordination \\
\arrayrulecolor{black!18}\specialrule{0.15pt}{3pt}{3pt}\arrayrulecolor{black}
% Author-supplied protocol (2026-09-25); local implementation validation remains pending.
% Initialization: launch Aimlabs, search for Gridshot 3x3, wait 10 s for results,
% select the first result by whoisaqua, start training, and wait 3 s before handoff.
\gameicon{steam_714010.jpg}{Aimlab 2.0 (AIM)} & Shoot as many blue targets as possible in 30-s Gridshot 3x3 by whoisaqua; three targets are visible, with each hit target replaced & One point per target destroyed; misses earn zero. OCR reads the final target-kill count from the results screen & Visual target localization; precise aiming and rapid shooting \\
\arrayrulecolor{black!18}\specialrule{0.15pt}{3pt}{3pt}\arrayrulecolor{black}
\gameicon{steam_1623730.jpg}{Palworld (PAL)} & Explore a dungeon and capture two target creatures & Captures earn points; early captures add bonuses; wasted balls incur penalties & Exploration; combat and capture planning \\
\addlinespace[4pt]
\bottomrule
\end{tabular}
\end{table}
% Elden Ring remains a candidate outside this provisional fifteen-game layout.

\clearpage
\section{Case Studies}
\label{app:program-cases}
These cases analyze how coding agents revise perception, feedback, and control logic before selecting a frozen program. G levels describe the use of game information, and modification-depth badges describe changes between adjacent displayed archives using the rubric in the Evaluation Measures section of the main paper; no aggregate IMS is computed for these illustrations. Screenshots provide context for the program analysis.

\subsection{Slay the Spire: Selecting an Earlier Program}
\label{app:case-slay}
Program selection need not favor the latest revision. Figure~\ref{fig:slay-the-spire-case-study} follows seven revisions from a minimal fallback through visual combat control, map probing, and room handling. After further revisions and retests, the agent selected the earlier v4 archive (\texttt{79f0903e8ef7}).

The map routine makes the role of feedback concrete. It probes candidate nodes, checks for a visual response, waits for a transition, and verifies that the map has disappeared before treating a click as successful. Generic room handling similarly rotates candidate clicks after unsuccessful attempts and reclassifies the resulting screen. These checks encode a reusable interaction procedure: issuing an input alone is insufficient to establish that the intended transition occurred. The later attack-priority, probe-cursor, and turn-gating revisions modify different parts of this procedure.

The return to v4 separates code revision from artifact selection. Additional edits did not compel selection of the newest program. The selected artifact preserves one particular combination of combat, map, and room-handling routines from the development trajectory.

\begin{figure}[!ht]
\centering
\includegraphics[width=\linewidth]{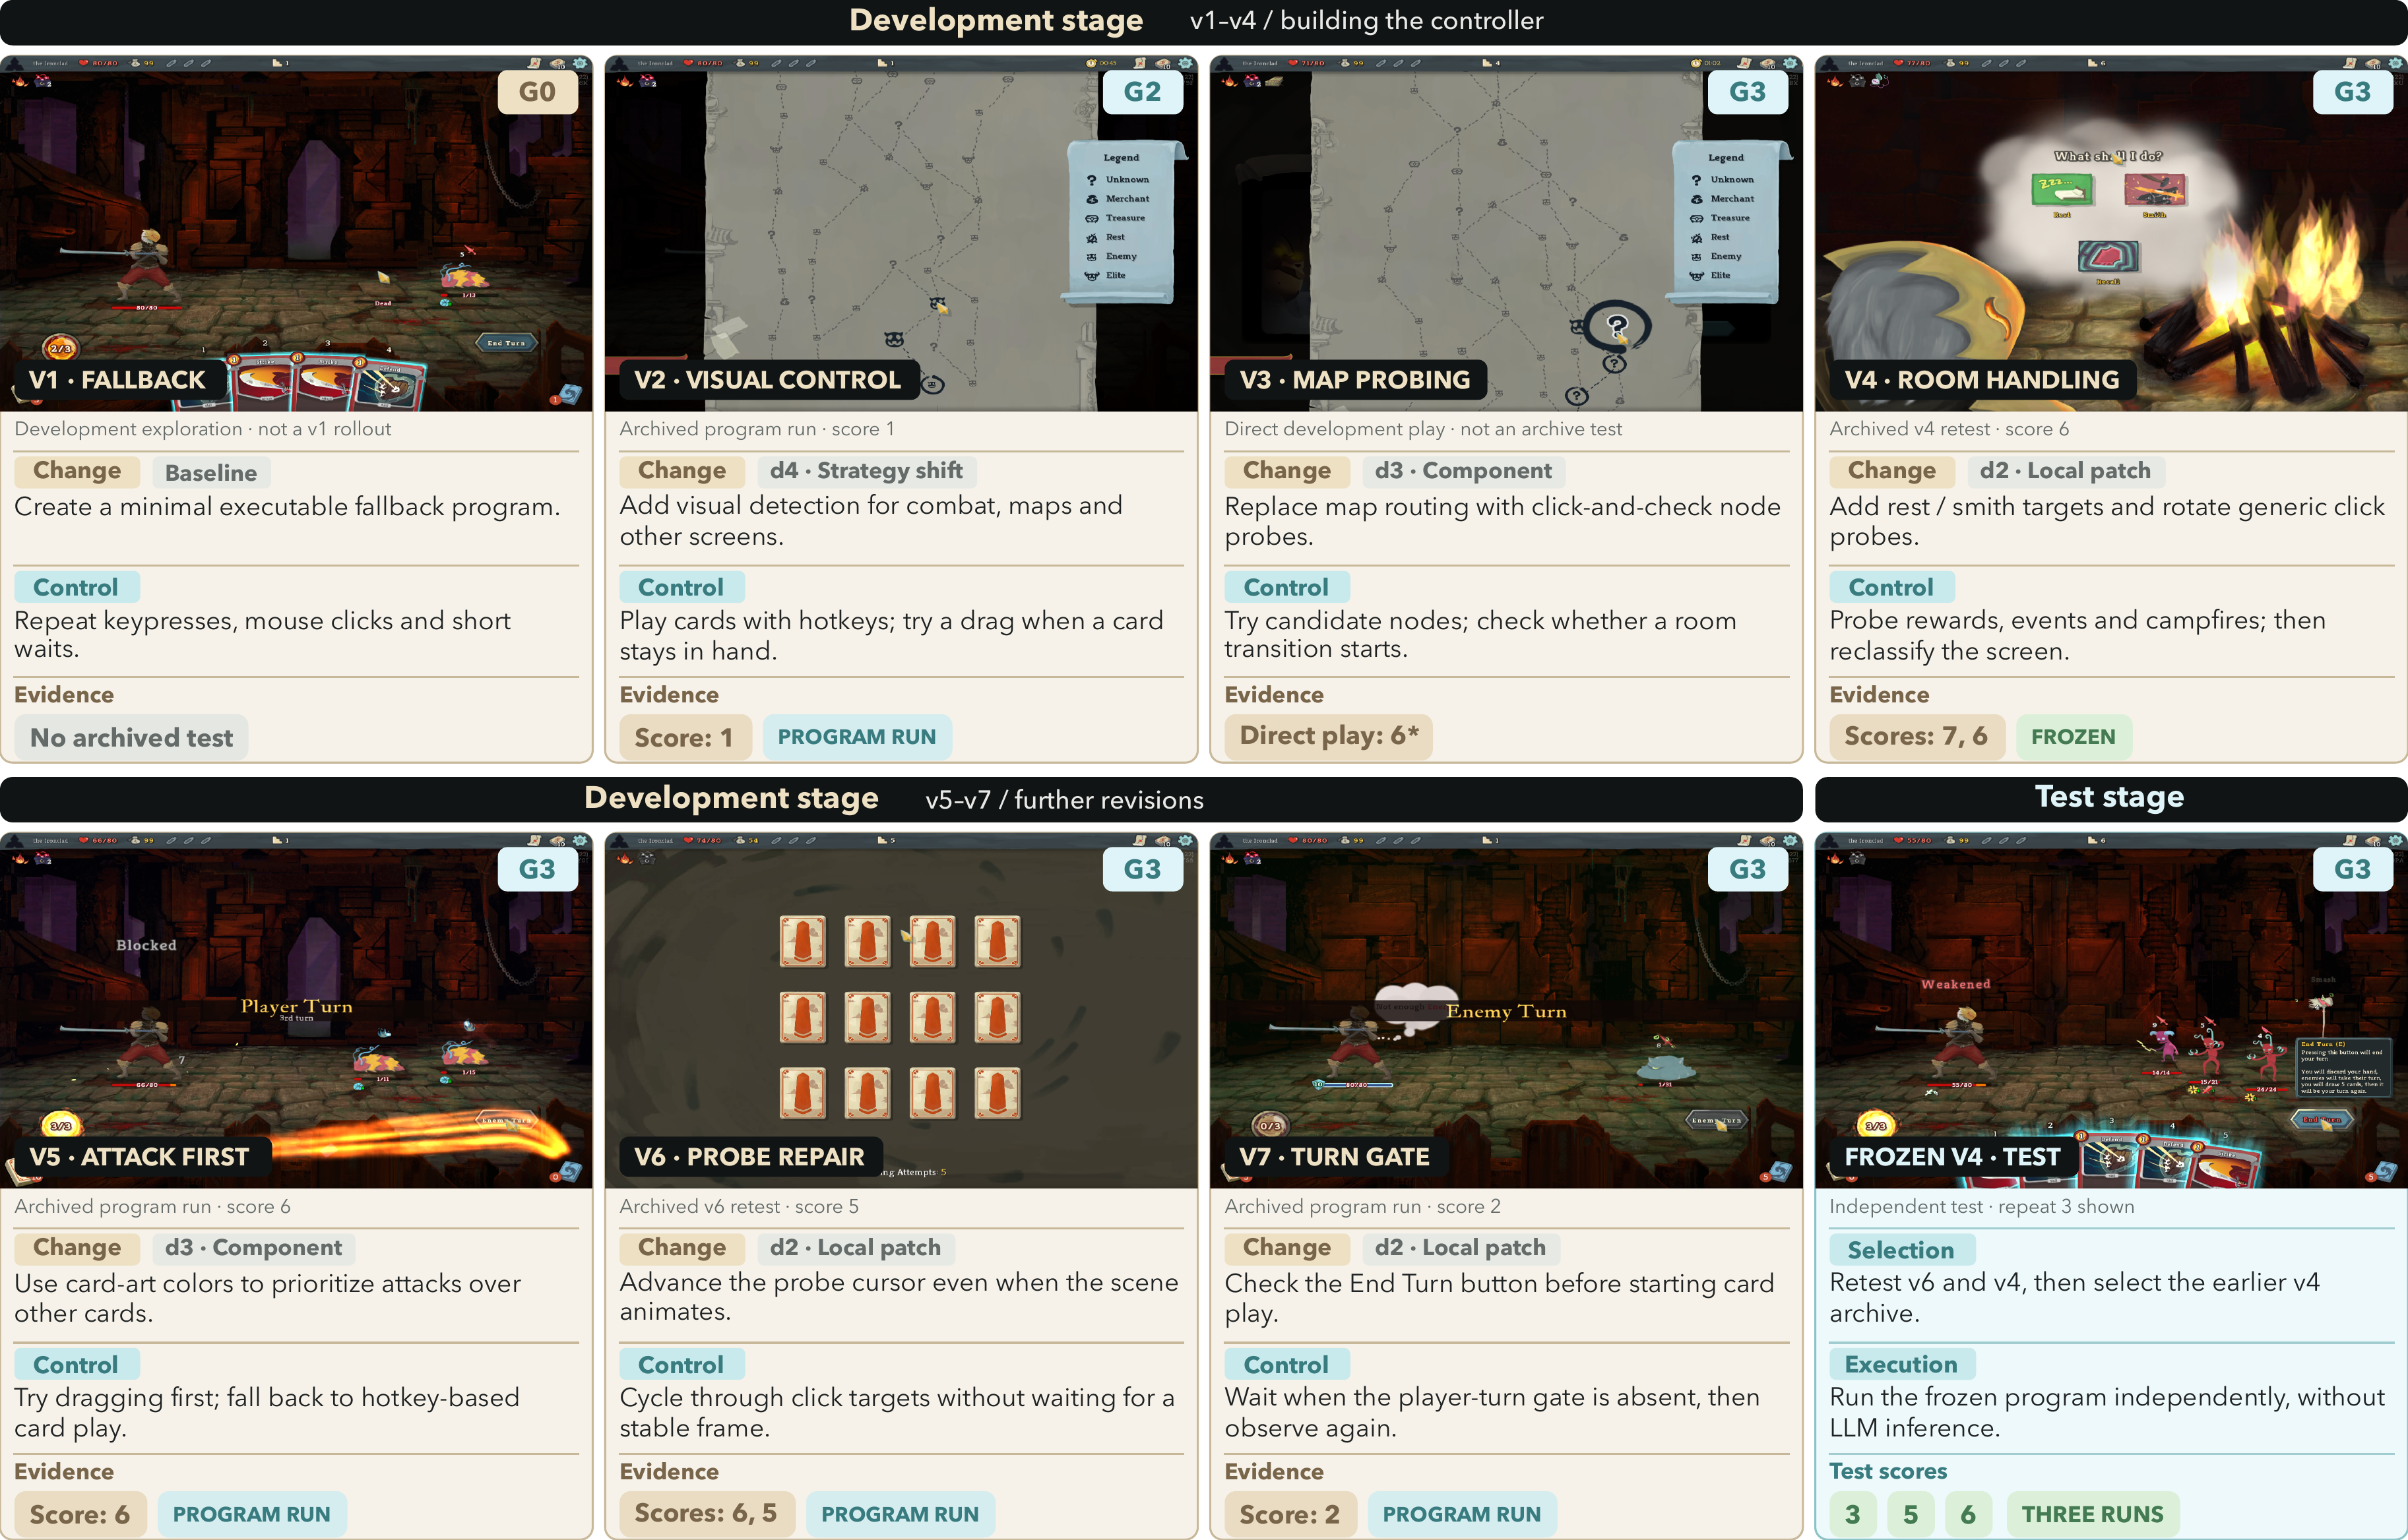}
\caption{\textbf{Program development and selection in \textit{Slay the Spire}.}
Seven revisions led to frozen v4. G labels indicate grounding; Change badges apply the IMS depth rubric to adjacent archives: d2, local patch; d3, component change; d4, strategy shift. v1 is the baseline. Scores are individual runs; v1 shows exploration, and v3's starred score is from direct play. v2 groups two snapshots.}
\label{fig:slay-the-spire-case-study}
\end{figure}

\clearpage

\subsection{Forza Horizon 5: Revising Perception and Recovery}
\label{app:case-forza}
The Claude Opus 5 driver turns minimap observations into steering and recovery decisions. Figure~\ref{fig:forza-case-study} shows revisions to the signals used by these decisions, followed by selection of v10 (\texttt{d5035a5b764b}) after a v11 lookahead experiment.

Two changes address different sources of ambiguity. Main-view frame differences can reflect scene animation as well as vehicle movement; minimap displacement provides a more specific motion signal for the implemented stall detector. Separately, radial groups of route pixels can mix nearby portions of a winding route. Connected-route tracing instead orders pixels by distance along the detected route before estimating near and far bearings. These are changes to the information used for control, while v11's altered bearing weights change how the same estimates influence steering.

The trajectory also includes reversals in design: v8 restores the earlier control law while retaining minimap-based stall detection, and the final selection returns from v11 to v10. This illustrates development as revising and recombining executable components.

\begin{figure}[!ht]
\centering
\includegraphics[width=\linewidth]{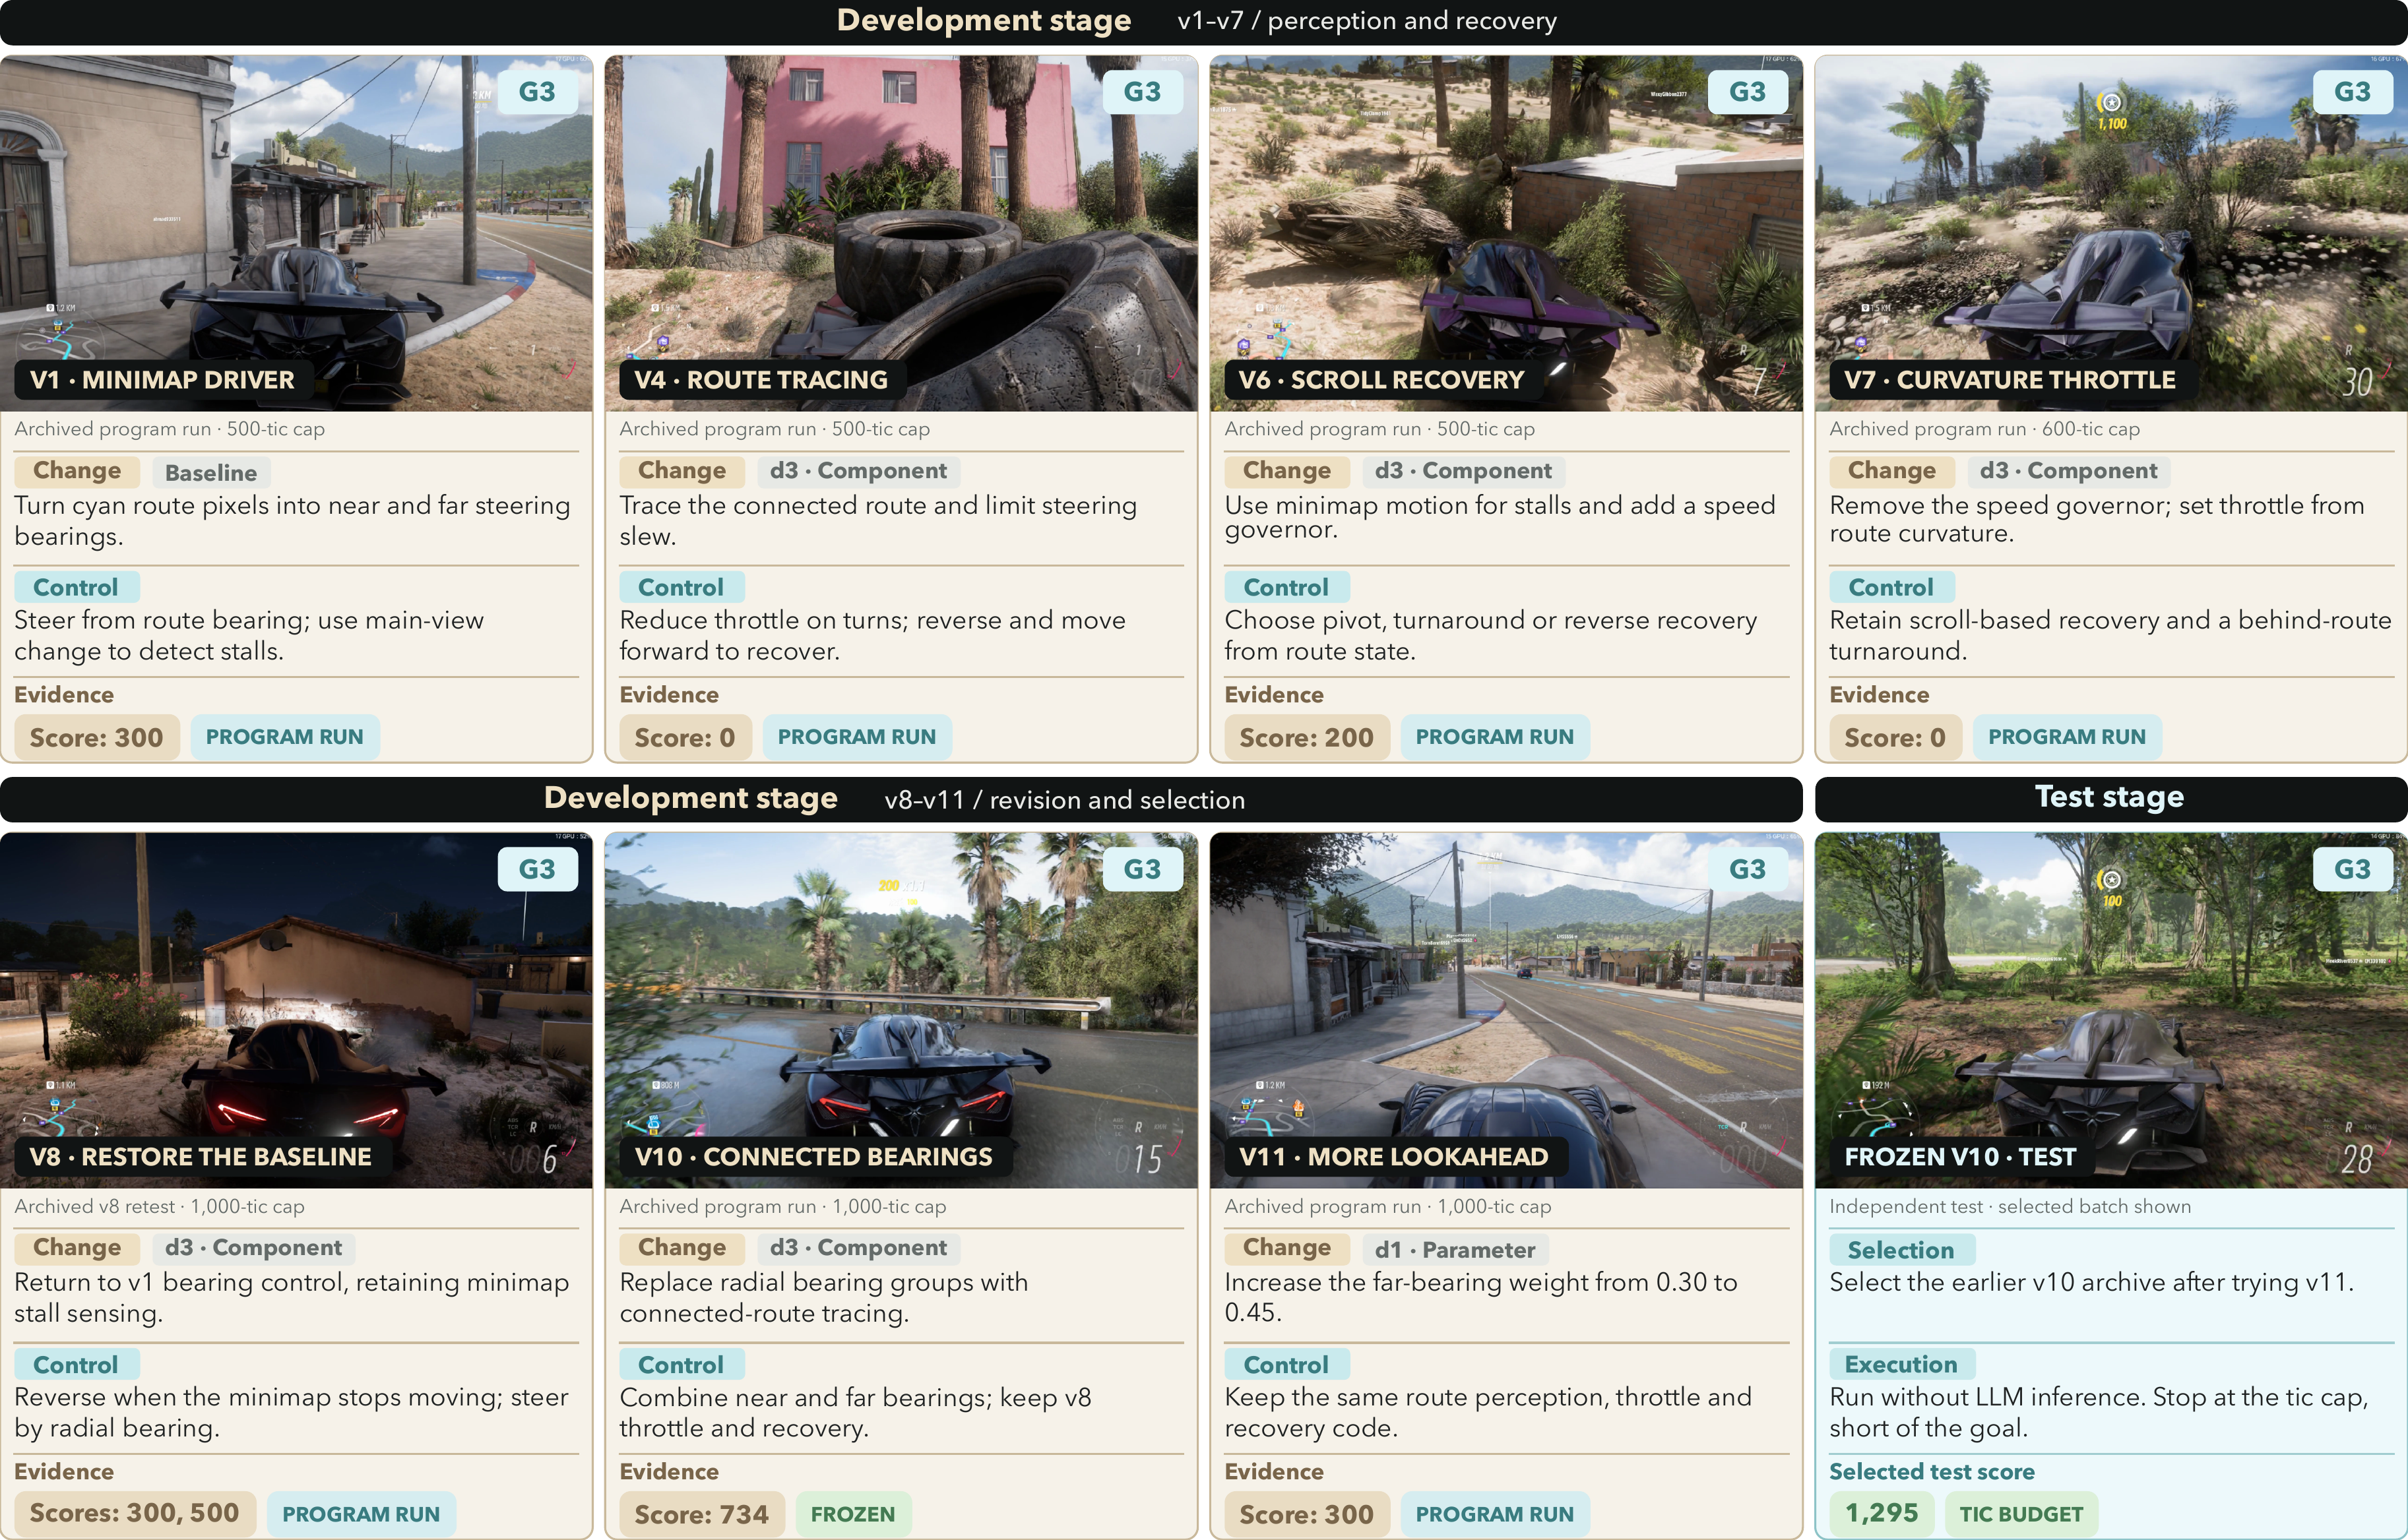}
\caption{\textbf{Program development and selection in \textit{Forza Horizon 5}.} Seven selected revisions illustrate changes to route perception, stall detection, and steering before selection of frozen v10; v9's throttle experiment is omitted. v8 retains minimap-based stall detection while restoring the earlier control law. The final selection returns from the v11 lookahead experiment to v10.}
\label{fig:forza-case-study}
\end{figure}

\clearpage

\subsection{BattleBlock Theater: Revising the Signal for Progress}
\label{app:case-battleblock}
A controller must distinguish visible motion from useful progress. In Figure~\ref{fig:battleblock-case-study}, the Claude Opus 5 program moves from fixed traversal to camera-motion feedback and persistent recovery state. The agent selects v5 (\texttt{f4d89e0b7753}) as the frozen program.

The transition from v4 to v5 exposes a specific interaction between recovery rules. In v4, vertical motion can reduce the same stall counter that eventually triggers direction reversal. Repeated jumping can therefore postpone reversal even without horizontal advance. v5 separates these signals: vertical motion still affects local recovery, but a distinct dead-end counter accumulates absent horizontal progress and reverses direction after 16 observations. The code change preserves the existing jump and back-off routines while changing when the controller abandons its current direction.

This revision makes horizontal progress a separate control signal, so vertical movement no longer prevents the controller from abandoning a blocked direction. The budget-guard revision separately accounts for execution limits. Development and independent testing use a per-episode limit of 3,000 game tics.

\begin{figure}[!ht]
\centering
\includegraphics[width=\linewidth]{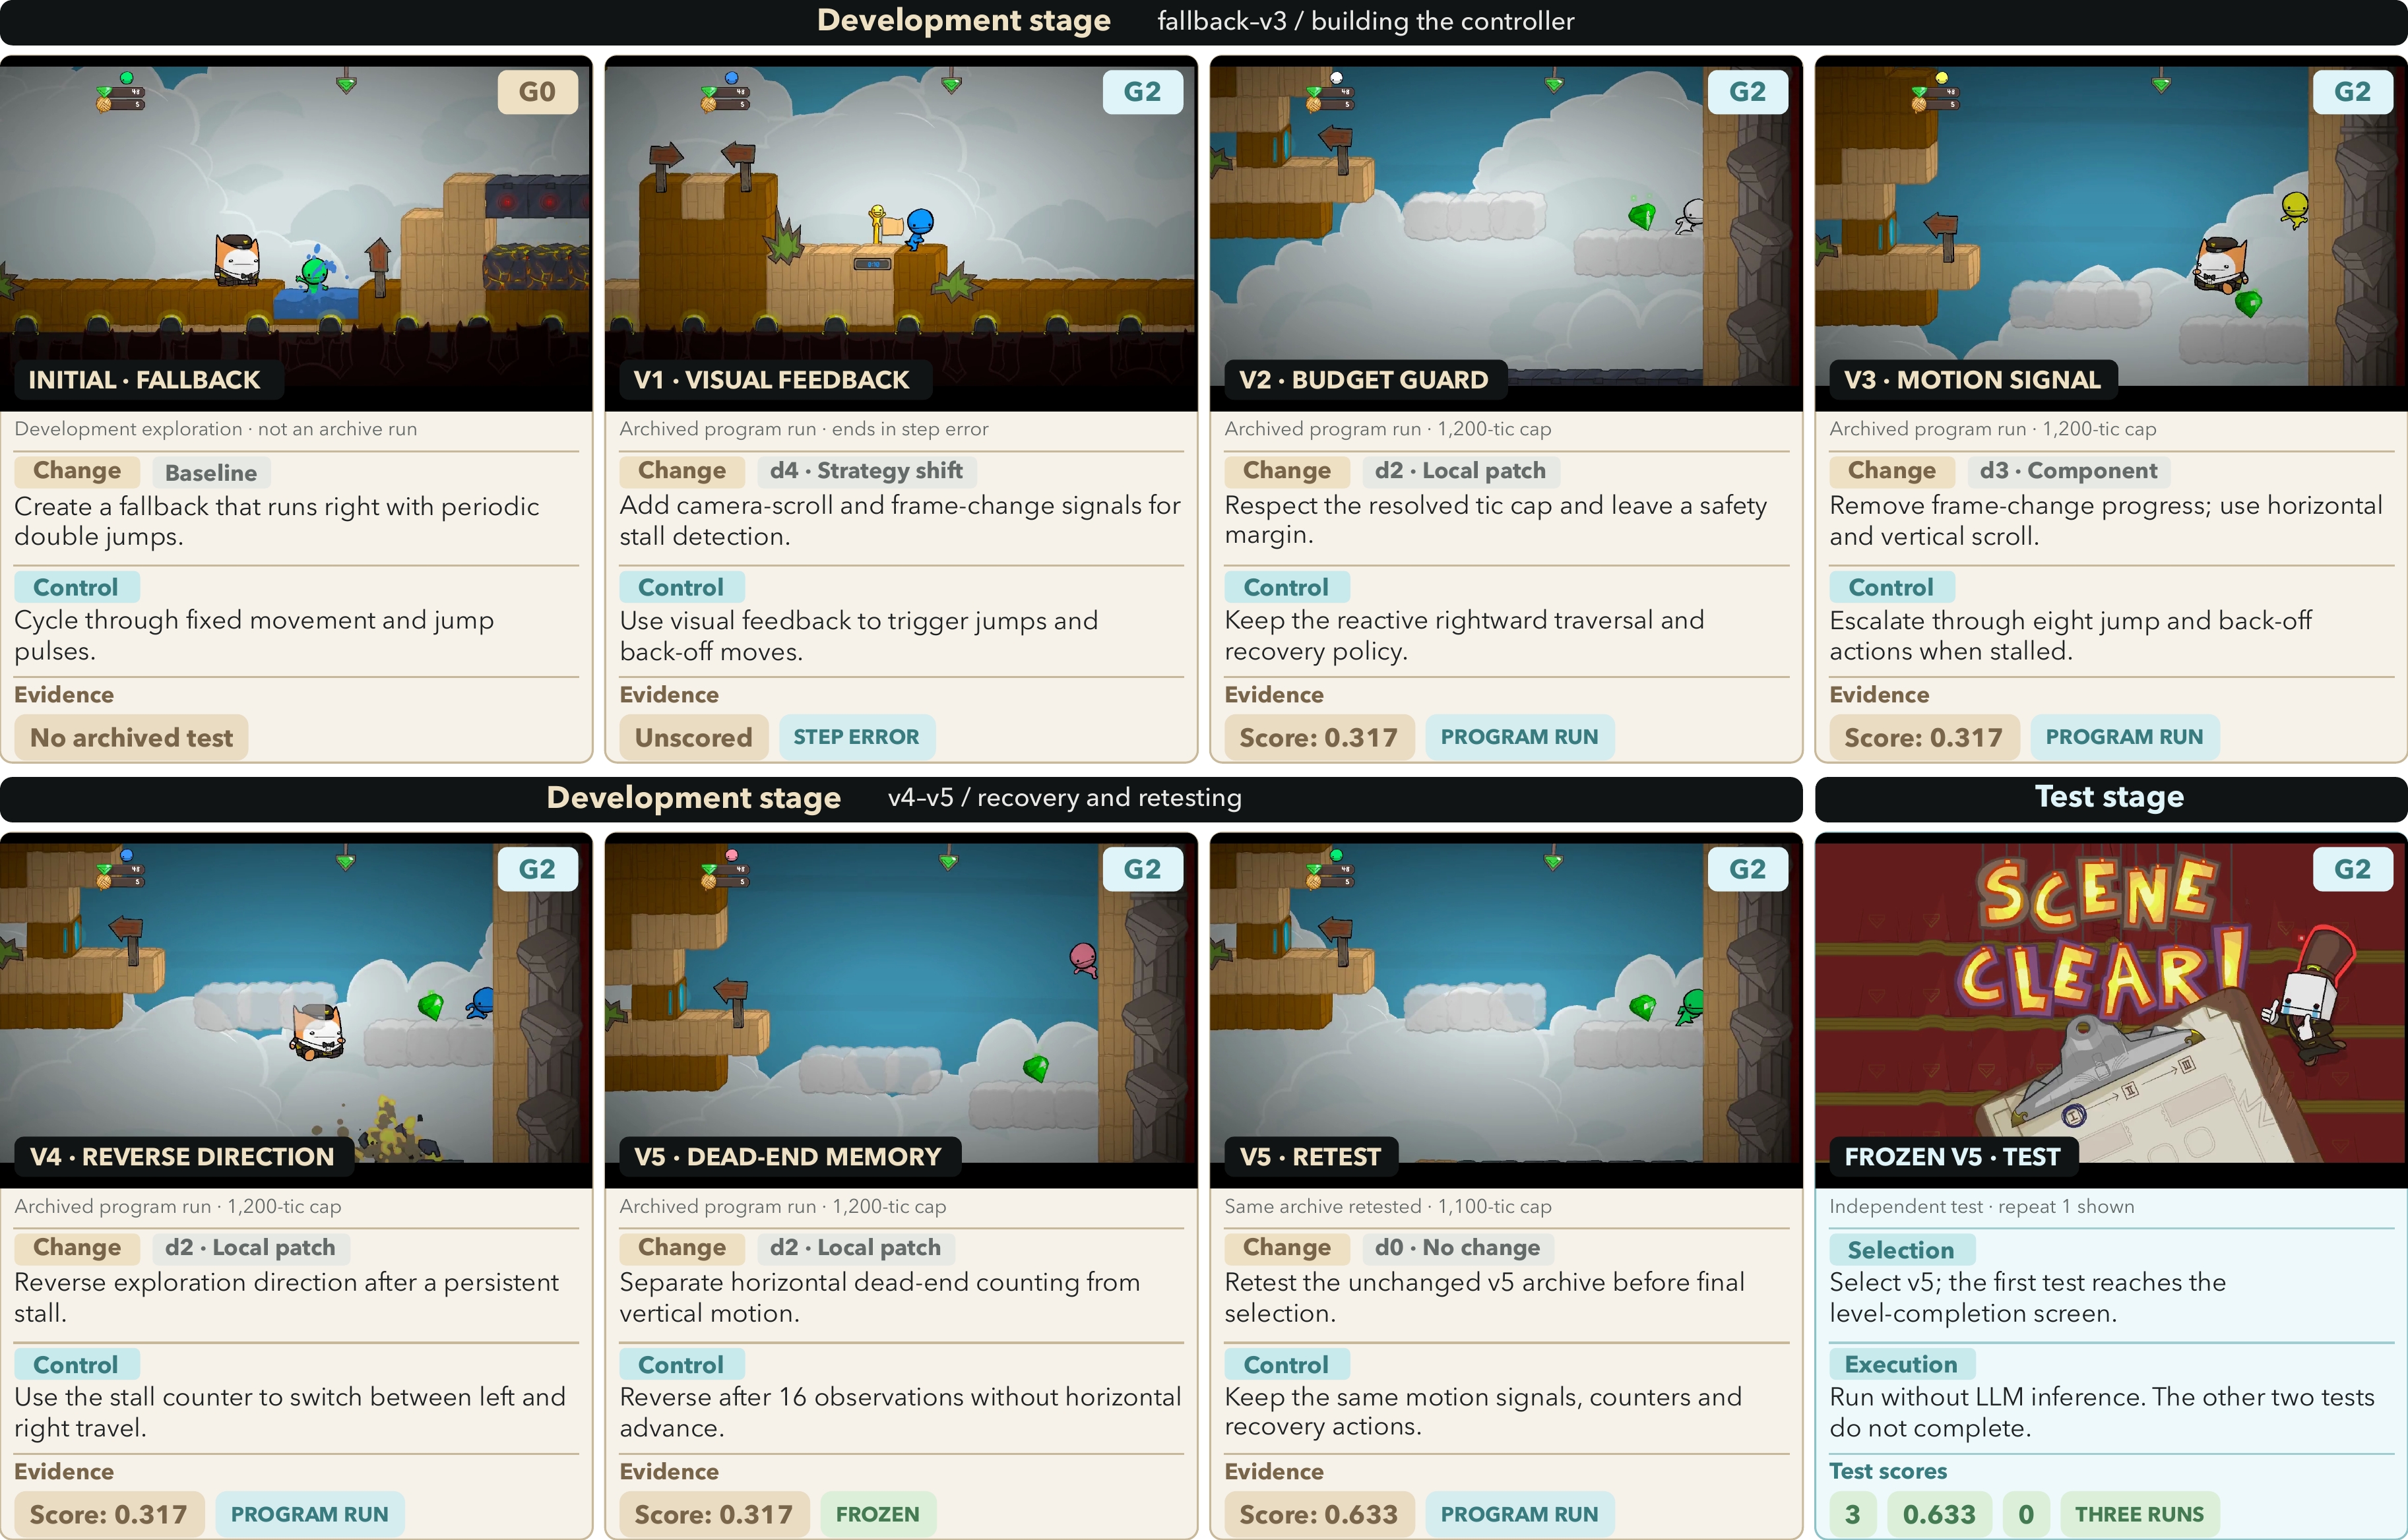}
\caption{\textbf{Program development and testing in \textit{BattleBlock Theater}.} The initial screenshot shows development exploration; subsequent panels illustrate program runs. Revisions add visual feedback, budget handling, motion signals, and persistent recovery state before selection of v5. Development and independent testing use a 3,000-game-tic episode limit.}
\label{fig:battleblock-case-study}
\end{figure}

\clearpage

\subsection{Black Myth: Wukong: Revising Feedback and Action Timing}
\label{app:case-black-myth}
The Qwen3.8 Flash controller illustrates how coding makes state interpretation and action timing explicit. Figure~\ref{fig:black-myth-case-study} traces HUD-based combat control, healing feedback, and opening-sequence revisions. After testing later variants, the agent selected v8 (\texttt{6a2980c43be9}).

The revisions address both what the controller observes and when it observes again. v2 retains prior bar estimates when the HUD is absent instead of treating missing pixels as empty resources. v3 checks subsequent health readings to limit unsuccessful healing retries, while v8 inserts waits after healing inputs. These rules encode a distinction between issuing an action and observing its effect, although retaining old estimates can also leave the controller with stale state. v9 changes another aspect of feedback: batching three attacks postpones the next observation until the burst finishes.

The opening gate exposes a concrete control-flow issue. In v10, initial lock acquisition precedes the new gate; v11 moves that branch below it so opening actions occur first. This repair changes executable behavior even though both versions describe an opening gate. The final return to v8 shows that additional revisions need not determine the submitted artifact.

\begin{figure}[!ht]
\centering
\includegraphics[width=\linewidth]{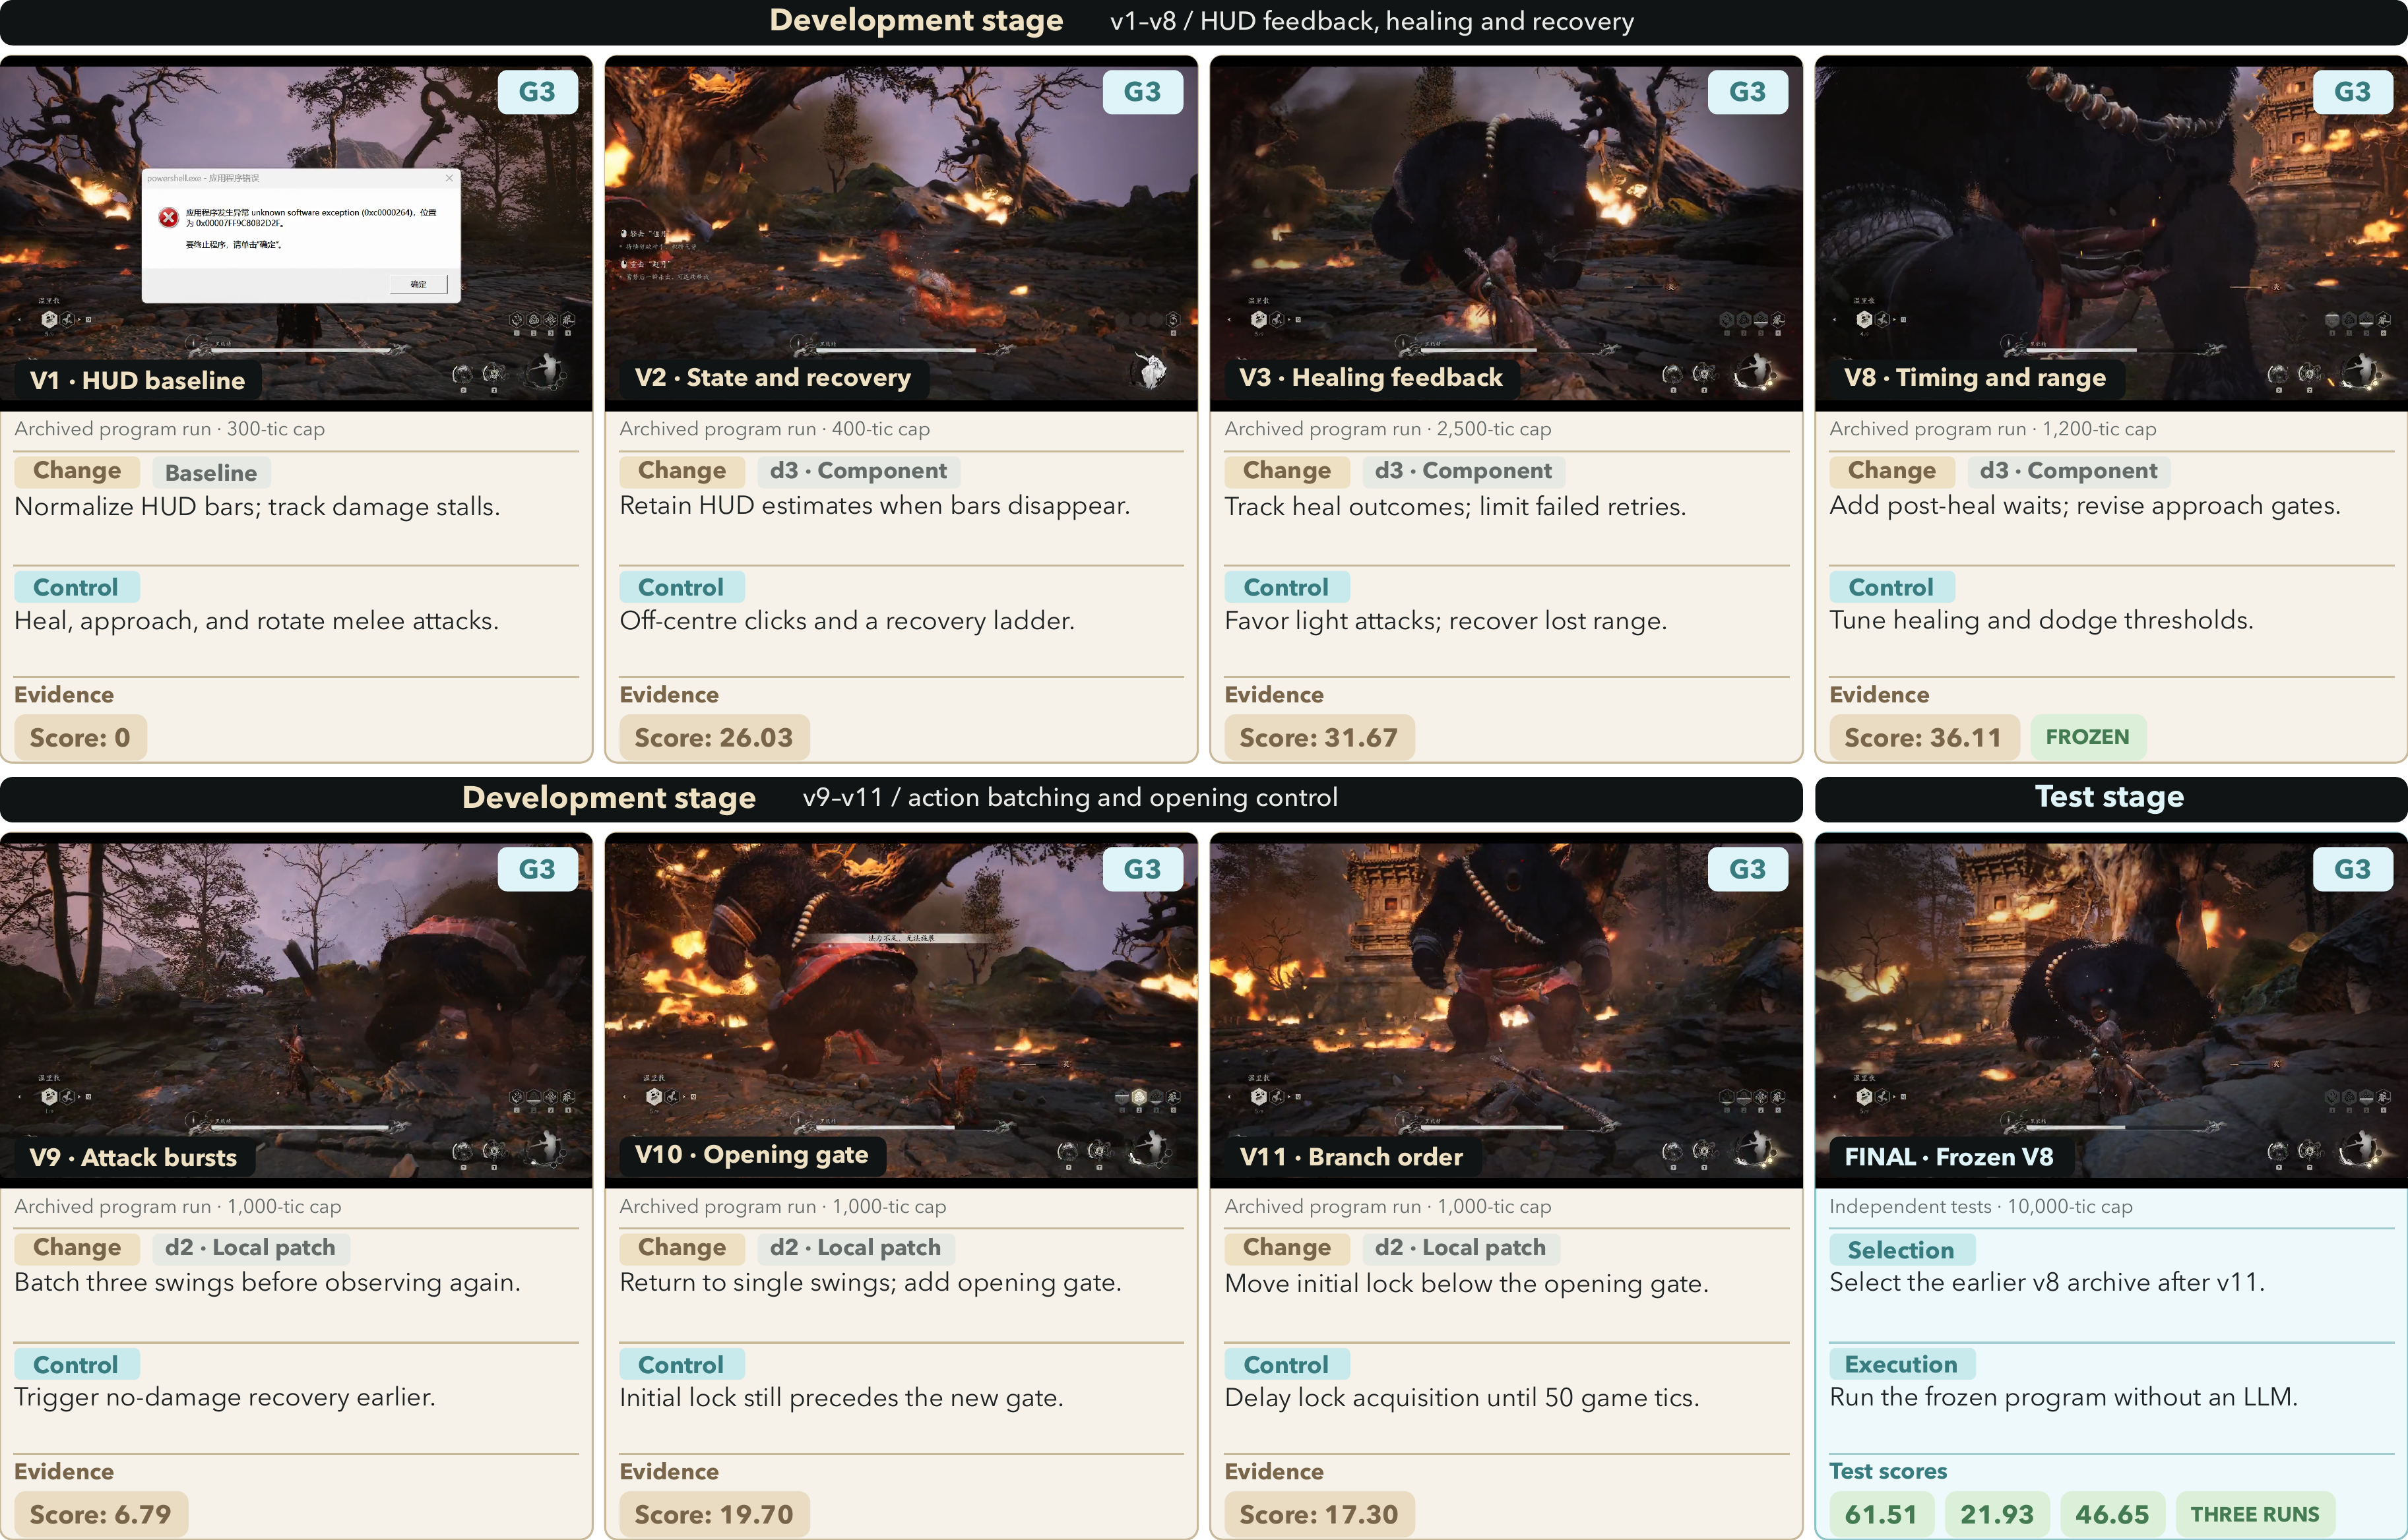}
\caption{\textbf{Program development and selection in \textit{Black Myth: Wukong}.} Seven selected archives illustrate revisions to HUD interpretation, healing feedback, action timing, and opening control flow; v4, v5, and v7 are omitted. The agent selects v8 after exploring later variants. The final panel shows execution of the selected frozen program.}
\label{fig:black-myth-case-study}
\end{figure}
